# Supplementary material for: PDBench: Evaluating Computational Methods for Protein Sequence Design
Source: arXiv:2109.07925 source file (2021-09-28)
Supplement: Supplementary file 1 [file appendix.tex]

\section{Appendix}

\subsection{Benchmark set}
\subsection{DNN model architectures}
